# Supplementary material for: Mechanical activity enables patterning and discrimination at the immune synapse
Source: arXiv:2510.18771 ancillary file (2025-10-21)
Supplement: Supplementary file 1 [file SI.pdf]

# Supplemental Material:
# Mechanical activity enables patterning and discrimination at the immune synapse


Tony Wong[1], Tom Chou[1,2], Suraj Shankar[3],[*] and Shenshen Wang[4†]

[1] *Department of Mathematics, University of California, Los Angeles, Los Angeles, CA, 90095-1555, USA*

[2] *Department of Computational Medicine, University of California, Los Angeles, Los Angeles, CA, 90095-1766, USA*

[3] *Department of Physics, University of Michigan, Ann Arbor, MI 48109, USA and*

[4] *Department of Physics and Astronomy, University of California, Los Angeles, Los Angeles, CA 90095, USA*


**Contents**


I. Model derivation & analysis 1

A. Nondimensionalized model 4

B. Parameter estimates 4

C. Effective free energy and linear stability analysis 5

II. Numerical simulation methods 7

III. Post-processing 8

IV. Supplementary Movies 10

References 11


## I. Model derivation & analysis

We build a minimal spatiotemporal model of patterning within an immune synapse by coupling the kinetics of receptor binding with the mechanics of membrane deformations and cytoskeletal activity of the immune cell. As the geometry of cellular contact is slender and fluid filled, we consider the gap between the cell membranes (the synaptic cleft) to be a thin lubricated fluid layer. Inertia is negligible on these scales as the Reynolds number Re $\ll 1$. Membrane deformations then drive squeezing flows in the gap, causing membrane relaxation to be governed by slow fluid drainage. Our derivation follows the elastohydrodynamic description in Ref. [1] and extends their passive model by including active forces (lateral and normal) along with feedback.

Within a lubrication approximation [2], the fluid stress is dominated by its pressure $p(\mathbf{x},t)$. Upon depth averaging through the gap thickness, force balance (Stokes' equation) in the fluid is dominated by viscous shear in the vertical direction that balances horizontal pressure gradients. Along with fluid incompressibility, this dictates

$$\partial_t h + \boldsymbol{\nabla}\cdot(h\mathbf{v}_f) = 0\ , \quad \mathbf{v}_f = -\frac{h^2}{12\eta}\boldsymbol{\nabla} p\ , \tag{1}$$

where $\mathbf{v}_f(\mathbf{x},t)$ is the depth-averaged flow velocity in the gap and $h(\mathbf{x},t)$ is the is the distance of the immune cell membrane from the antigen presenting surface (assumed flat). We assume the membrane is not permeable to the fluid and the velocity obeys a no-slip condition at the boundaries.

The fluid pressure is dictated by vertical force balance on the lymphocyte (B or T cell) membrane, which gives

$$-p = \gamma_0\nabla^2 h - B\nabla^4 h - k_R(h-\ell_R)c_R - k_A(h-\ell_A)c_A + \sigma_\perp^a\ , \tag{2}$$

where $\gamma_0$ is the membrane tension and $B$ is the bending modulus. Typical values of $\gamma_0 \sim 700\ k_BT/\mu\text{m}^2$ and $B \sim 400\ k_BT$ [1, 3, 4] show that membrane deformations on length scales comparable and larger than $\sqrt{B/\gamma_0} \sim 0.75\ \mu$m


[*] surajsh@umich.edu

[†] shenshen@physics.ucla.edu

are dominated by tension alone. So for simplicity, we neglect membrane bending rigidity and only retain a finite tension $\gamma_0$. The bound receptor-ligand complex is assumed to be a Hookean springs with stiffness $k_R$ and equilibrium length $\ell_R$, and the concentration of the bound receptor complex is $c_R(\mathbf{x}, t)$. Similarly, longer adhesion molecules with concentration $c_A(\mathbf{x}, t)$ have a rest length $\ell_A$ and an elastic stiffness $k_A$. Note that, vertical force balance (Eq. 2) can be written as $-p = -\delta\mathcal{F}/\delta h + \sigma^a_\perp$, i.e., the normal stress jump across the membrane is balanced by passive elastic forces [5] that derive from a free energy

$$\mathcal{F} = \frac{1}{2}\int \mathrm{d}^2x \left[B(\nabla^2 h)^2 + \gamma_0|\boldsymbol{\nabla} h|^2 + k_R c_R (h - \ell_R)^2 + k_A c_A (h - \ell_A)^2\right] . \tag{3}$$

In Eq. 2, the remaining normal stress ($\sigma^a_\perp$) on the membrane is exerted by the actomyosin cortex from within the cell. On time scales longer than the turnover time of the cortical network, we can model the actomyosin cortex as a thin active fluid layer [6, 7]. The cortical active stress (in 3D), $\boldsymbol{\sigma}^a$, is taken to be uniaxially anisotropic in the $z$-direction and isotropic in the 2D plane (parallel to the membrane surface), neglecting any orientational order in the plane. Setting $\sigma^a_{xz} = \sigma^a_{yz} = 0$, we write the in-plane 2D active stress as $\boldsymbol{\sigma}^a_\parallel = \alpha m\mathbf{I}$ and the vertical active stress component as $\sigma^a_{zz} \equiv \sigma^a_\perp = \zeta[m - \langle m\rangle]$, where $\langle m\rangle(t) = (1/\pi R^2)\int \mathrm{d}\mathbf{x}\, m(\mathbf{x}, t)$ is the spatial average. The active stress depends on the local fraction of bound/phosphorylated actomyosin units $m(\mathbf{x}, t)$ and contractility $\alpha > 0$ captures the average (contractile) force dipole exerted by the molecular motors, while $\zeta > 0$ captures active pulling by a cortical (normal) force density. In general $\alpha \neq \zeta$, allowing active forces of different strengths to be exerted in horizontal and vertical directions. Furthermore, to prevent global delamination of the membrane from strong pulling, we choose $\sigma^a_\perp$ to be globally (but not locally) balanced, i.e., $\int \mathrm{d}\mathbf{x}\, \sigma^a_\perp = 0$, so when $m$ is spatially homogeneous, there is no active pulling, as expected for an unpatterned cell membrane. Note that including a similar spatially constant offset in $\boldsymbol{\sigma}^a_\parallel$ is irrelevant, as only its gradients are important (see below).

As the cortex is far more viscous than the cell membrane [8], tangential force balance is dominated by cortical flows ($\mathbf{v}_c(\mathbf{x}, t)$) and stresses ($\boldsymbol{\sigma}^a_\parallel$), which gives

$$-\Gamma\mathbf{v}_c + \boldsymbol{\nabla}\cdot\boldsymbol{\sigma}^a_\parallel = \mathbf{0} \implies \mathbf{v}_c = \frac{\alpha}{\Gamma}\boldsymbol{\nabla} m . \tag{4}$$

For simplicity, we have assumed a Darcy-like description for viscous friction due to permeation through a porous actomyosin network or the finite cortical thickness that frictionally screens viscous flows. The effective cortical friction $\Gamma \sim \max(\mu_{\mathrm{cortex}}/\ell_c^2, \mu_{\mathrm{cytosol}}/\ell_p^2)$ is dictated by either the cortex viscosity $\mu_{\mathrm{cortex}} \sim 10 - 100$ Pa s and layer thickness $\ell_c \sim 200 - 300$ nm [8, 9] or the cytosolic viscosity $\mu_{\mathrm{cytosol}} \sim 10^{-3} - 10^{-2}$ Pa s and actomyosin pore size $\ell_p \sim 15 - 20$ nm [10]. Based on these estimates, we expect the dominant contribution is from cortex visco(elasticity), which yields $\Gamma \sim \mu_{\mathrm{cortex}}/\ell_c^2 \sim 10^2 - 10^3$ Pa s/$\mu$m$^2$.

Finally, the turnover of actomyosin units is governed by a simple kinetic equation (neglecting gradient terms) $\partial_t m = r_{\mathrm{on}}(1 - m) - r_{\mathrm{off}} m$. We invoke a simple, biologically motivated [11] feedback rule that local contractile units are recruited when the receptor binds, i.e., $r_{\mathrm{on}}(c_R) = r^0_{\mathrm{on}}(1 + \chi c_R)$ with $\chi > 0$ as the simplest linear dependence, and take $r_{\mathrm{off}}$ to be a constant. By assuming rapid relaxation of actomyosin kinetics and neglecting the time taken for active stresses to build-up, we set $\partial_t m = 0$ to obtain

$$m = \frac{r_{\mathrm{on}}(c_R)}{r_{\mathrm{on}}(c_R) + r_{\mathrm{off}}} = m_0\left(\frac{1 + c_R\chi}{1 + m_0\chi c_R}\right) , \tag{5}$$

where we obtain a simple Michaelis-Menten style saturating response curve for $m$ by writing $m_0 = r^0_{\mathrm{on}}/(r^0_{\mathrm{on}} + r_{\mathrm{off}})$ as the basal pool of myosin present even in the absence of any bound receptors ($c_R = 0$).

Eqs. 1, 2, and 4 collectively enforce mass and force balance (vertical and horizontal) in the system. We next describe how the chemical kinetics of receptor and adhesion molecules is modeled.

The molecular dynamics of the transmembrane proteins (labeled by $i = R, A$, where $R$: receptor molecules and $A$: adhesion molecules) includes binding-unbinding kinetics governed by transition rates $\omega^i_{\mathrm{on}}$ (binding) and $\omega^i_{\mathrm{off}}$ (unbinding) and transport by passive molecular diffusion ($D_i$ is a diffusion constant), advection by cortical active flows $\mathbf{v}_c$, and passive dissipative flows $-(D_i/k_BT)\delta\mathcal{F}/\delta c_i$ due to the elastic tethering to the membrane (required by thermodynamic consistency, see [1, 12]). Putting these all together, we obtain

$$\partial_t c_R + \boldsymbol{\nabla}\cdot(c_R\mathbf{v}_c) = \omega^R_{\mathrm{on}}(c^0_R - c_R) - \omega^R_{\mathrm{off}} c_R + D_R\boldsymbol{\nabla}\cdot\left[\boldsymbol{\nabla} c_R + \frac{c_R}{k_BT}\boldsymbol{\nabla}\frac{\delta\mathcal{F}}{\delta c_R}\right] , \tag{6}$$

$$\partial_t c_A + \boldsymbol{\nabla}\cdot(c_A\mathbf{v}_c) = \omega^A_{\mathrm{on}}(c^0_A - c_A) - \omega^A_{\mathrm{off}} c_A + D_A\boldsymbol{\nabla}\cdot\left[\boldsymbol{\nabla} c_A + \frac{c_A}{k_BT}\boldsymbol{\nabla}\frac{\delta\mathcal{F}}{\delta c_A}\right] , \tag{7}$$

where $c_R^0$ and $c_A^0$ are the equilibrium concentrations of bound receptor-antigen complexes and bound adhesion molecules, respectively.

The kinetic rates encode geometric and mechanical mechanisms of feedback ($\omega^i_{\mathrm{on/off}}(h)$, $i = R, A$) through their dependence on the membrane height. Neglecting active/nonequilibrium processes in the kinetics (phosphorylation dependent kinetic proofreading steps being downstream in activation [13]), the rates obey detailed balance, hence

$$\frac{\omega^R_{\mathrm{on}}}{\omega^R_{\mathrm{off}}} = e^{-\Delta E_R(h)/k_BT} \ , \quad \Delta E_R(h) = \frac{k_R}{2}(h-\ell_R)^2 - E_b^R \ , \tag{8}$$

$$\frac{\omega^A_{\mathrm{on}}}{\omega^A_{\mathrm{off}}} = e^{-\Delta E_A(h)/k_BT} \ , \quad \Delta E_A(h) = \frac{k_A}{2}(h-\ell_A)^2 - E_b^A \ , \tag{9}$$

where $\Delta E_{R,A}(h)$ is the energy difference between the bound and unbound states of the receptor/antigen molecules and $E_b^{R,A}$ is the respective binding energy to the ligand, so $K^i_{\mathrm{eq}} = e^{E^i_b/k_BT}$ is the corresponding equilibrium binding affinity ($i = R, A$). Following Ref. [14], we estimate the individual kinetic rates using Kramer's theory and consider the transition state to binding to behave as spring with a different elastic stiffness ($k'_R$, $k'_A$). Then we obtain

$$\omega^R_{\mathrm{on}}(h) = \omega_R \, K^R_{\mathrm{eq}} \, e^{-k'_R(h-\ell_R)^2/(2k_BT)} \qquad \omega^R_{\mathrm{off}}(h) = \omega_R \, e^{(k_R-k'_R)(h-\ell_R)^2/(2k_BT)} \ , \tag{10}$$

$$\omega^A_{\mathrm{on}}(h) = \omega_A \, K^A_{\mathrm{eq}} \, e^{-k'_A(h-\ell_A)^2/(2k_BT)} \qquad \omega^A_{\mathrm{off}}(h) = \omega_A \, e^{(k_A-k'_A)(h-\ell_A)^2/(2k_BT)} \ , \tag{11}$$

where $\omega_{R,A}$ set overall kinetic timescales. The kinetic rates encode geometric and mechanical mechanisms of feedback. If the transition state is stiffer than the bound state ($k'_i > k_i$) then $\omega^i_{\mathrm{off}} \to 0$ as $h \to \infty$, i.e., we have a catch-bond and the bound complex lifetime ($1/\omega^i_{\mathrm{off}}$) increases with load. Otherwise, when $k'_i < k_i$, we have a regular slip bond, and the bound complex breaks easily when loaded. Cellular adhesion, mediated by integrins, e.g., LFA-1-ICAM-1 bonds, typically form catch bonds [14–16], while immune receptors can form both catch-slip bonds, e.g., in TCRs, and slip bonds in BCRs [17–21]. Here for simplicity, we neglect such catch or slip behavior and simply set $k'_i = k_i$ for $i = R, A$, so that unbinding occurs at a constant rate ($\omega^i_{\mathrm{off}} = \omega_i$, a constant), and all $h$ dependence is then only present in the binding rates $\omega^i_{\mathrm{on}}$. Note that a catch/slip bond behavior modeled as in Eqs. 10, 11 does not affect the spatially homogeneous steady-state concentrations which only depends on the ratio $\omega^i_{\mathrm{on}}/\omega^i_{\mathrm{off}}$, that is fixed entirely by detailed balance (Eqs. 8, 9). In Sec. I C, we also see that including such catch/slip bond behavior does not affect the linear stability of a spatially homogeneous state, so its consequences must necessarily be nonlinear. For these reasons, we neglect the impact of catch/slip bond behavior here and leave that for a future study.

Eqs. 1-7 provide a complete dynamical model for synaptic patterning. But the model is still quite complex, with many parameters and multiple scales, making its numerical investigation challenging. A simplification is afforded by noting that the molecular kinetics occurs on a much faster time scale than the relaxation of membrane deformations. This time scale separation allows one to locally equilibrate the concentrations to their steady-state values $c_i \approx c_i^0 \omega^i_{\mathrm{on}}(h)/[\omega^i_{\mathrm{on}}(h) + \omega^i_{\mathrm{off}}]$, which depend on the membrane height through the nonlinear binding rates. This approximation works well in the passive case, where transport processes can be neglected, as previously shown in Ref. [4]. But when active transport is present and strong, this approximation breaks down, as activity can generate patterning instabilities on a fast kinetic timescale, preventing a local equilibration of the concentration. To still make progress and make the model computationally tractable, we adopt an intermediate simplification motivated by experimental observations. While bound receptors co-localize with actomyosin and generate local contractile stresses that can amplify clustering (feedback via Eq. 5 and see Refs. [11, 20]), adhesion molecules are usually excluded from these clusters and instead occupy regions with low actomyosin activity. This suggests that while the effect of cortical flows cannot be neglected in receptor dynamics, the role of cortical flows is likely weaker in adhesion dynamics. So to simplify our analysis, we neglect active flows and spatial gradients in Eq. 7 and equilibrate $c_A$ to its $h$-dependent steady-state value as

$$c_A = c_A^0 \frac{\omega^A_{\mathrm{on}}(h)}{\omega^A_{\mathrm{on}}(h) + \omega^A_{\mathrm{off}}} = \frac{c_A^0}{1 + e^{\Delta E_A(h)/k_BT}} \ , \tag{12}$$

and only retain explicit dynamics for the receptors (Eq. 6). This simplification is only to make the problem computationally tractable and reduce the number of parameters; further work is needed to establish the broader validity of these assumptions and approximations.

Our final model thus incorporates only two dynamical fields, the membrane height ($h(\mathbf{x}, t)$) and the bound receptor density ($c_R(\mathbf{x}, t)$). It is convenient to write the dynamics of the latter in terms of the relative bound fraction $\rho(\mathbf{x}, t) = c_R(\mathbf{x}, t)/c_R^0$. Together, the simplified model coupling the kinetics of the receptors with the dynamics of the membrane

is then given by

$$\partial_t h = \boldsymbol{\nabla}\cdot\left(\frac{h^3}{12\eta}\boldsymbol{\nabla}p\right) \,, \tag{13a}$$

$$\partial_t \rho = \omega_{\rm on}^R(h)\,(1-\rho) - \omega_{\rm off}^R\,\rho + \boldsymbol{\nabla}\cdot\left[D_R\boldsymbol{\nabla}\rho + \frac{\rho k_R D_R}{k_B T}(h-\ell_R)\boldsymbol{\nabla}h - \frac{\alpha\rho}{\Gamma}\boldsymbol{\nabla}m\right] \,, \tag{13b}$$

$$p = -\gamma_0\nabla^2 h + k_R c_R^0\rho(h-\ell_R) + k_A\frac{c_A^0(h-\ell_A)}{1+e^{\Delta E_A(h)/k_BT}} - \zeta\left[m - \langle m\rangle\right] \,, \tag{13c}$$

$$m = m_0\left(\frac{1+c_R^0\rho\chi}{1+m_0c_R^0\chi\rho}\right) \tag{13d}$$

The model is completed upon specifying boundary conditions. We consider a circular contact zone and assume the membrane adopts an average height at the boundary $h|_R = h_0$ given by the weighted average of the receptor and adhesion molecule lengths, i.e., $h_0 = (c_R^0\ell_R + c_A^0\ell_A)/(c_R^0 + c_A^0)$. We allow free drainage of the fluid through the boundary by enforcing $p|_R = 0$ and assume zero diffusive flux of bound receptors, so $\hat{\boldsymbol{\nu}}\cdot\boldsymbol{\nabla}\rho|_R = 0$, where $\hat{\boldsymbol{\nu}}$ is the outward normal at the boundary.

### A. Nondimensionalized model

We nondimensionalize the variables in the following manner: $\tilde{t} = t/\tau_k$, $\tilde{\mathbf{x}} = \mathbf{x}/L_c$, $\tilde{\rho} = \rho/\rho_0$, and $\tilde{h} = h/h_0$. The relevant scales are the kinetic time scale $\tau_k = [\omega_{\rm on}^R(h_0) + \omega_{\rm off}^R]^{-1}$, the elasto-capillary like length scale $L_c = \sqrt{\gamma_0/(k_0c_R^0\rho_0)}$ and the average receptor bound fraction $\rho_0 = \omega_{\rm on}^R(h_0)\tau_k = K_{\rm eq}^R/[K_{\rm eq}^R + e^{E_0\epsilon_0^2}]$. The parameters $\epsilon_0 = (h_0-\ell_R)/h_0$ and $\epsilon_1 = (h_0-\ell_A)/h_0$ are measures of strain generated in the receptor/adhesion linker upon binding and $E_0 = k_Rh_0^2/(2k_BT)$ and $E_1 = k_Ah_0^2/(2k_BT)$ are dimensionless measures of the elastic energy in the receptors and adhesion molecules (relative to thermal energy) respectively.

Upon non-dimensionalization, we obtain

$$\mathsf{Eh}\;\tilde{\partial}_t\tilde{h} = \tilde{\boldsymbol{\nabla}}\cdot\left(\tilde{h}^3\tilde{\boldsymbol{\nabla}}\tilde{p}\right) \,, \tag{14}$$

$$\tilde{\partial}_t\tilde{\rho} = \tilde{\omega}_{\rm on}\left(\frac{1}{\rho_0} - \tilde{\rho}\right) - \tilde{\omega}_{\rm off}\,\tilde{\rho} + D\tilde{\boldsymbol{\nabla}}\cdot\left[\left(1 - \mathsf{Pe}\frac{\tilde{\rho}}{(1+\theta\tilde{\rho})^2}\right)\tilde{\boldsymbol{\nabla}}\tilde{\rho} + 2E_0\tilde{\rho}(\tilde{h}-1+\epsilon_0)\tilde{\boldsymbol{\nabla}}\tilde{h}\right] \,. \tag{15}$$

$$\tilde{p} = -\tilde{\nabla}^2\tilde{h} + \tilde{\rho}(\tilde{h}-1+\epsilon_0) + \frac{\kappa_0}{\rho_0}\frac{K_{\rm eq}^A(\tilde{h}-1+\epsilon_1)}{[K_{\rm eq}^A + e^{E_1(\tilde{h}-1+\epsilon_1)^2}]} - A_\zeta\left[\frac{\tilde{\rho}}{1+\theta\tilde{\rho}} - \left\langle\frac{\tilde{\rho}}{1+\theta\tilde{\rho}}\right\rangle\right] \,, \tag{16}$$

where $\kappa_0 = k_Ac_A^0/(k_Rc_R^0)$ is the weighted ratio of bond stiffness, $\theta = m_0\chi c_R^0$ controls the feedback nonlinearity, $\mathsf{Eh} = 12\eta/(k_Rc_R^0\rho_0h_0\tau_k)(L_c/h_0)^2$ is the elastohydrodynamic number, and active forces/flows are captured by $A_\zeta = m_0(1-m_0)\chi\zeta/(k_Rh_0)$ and $\mathsf{Pe} = \alpha m_0(1-m_0)\chi c_R^0\rho_0/(\Gamma D_R)$. The nondimensionalized kinetic rates are given by

$$\tilde{\omega}_{\rm on} = \rho_0\,e^{-E_0(\tilde{h}-1)(\tilde{h}-1+2\epsilon_0)} \,, \quad \tilde{\omega}_{\rm off} = (1-\rho_0) \,. \tag{17}$$

The boundary conditions are simply (at $\tilde{r} = \tilde{R} \equiv R/L_c$)

$$\tilde{h}|_{\tilde{R}} = 1 \,, \quad \tilde{p}|_{\tilde{R}} = 0 \,, \quad \hat{\boldsymbol{\nu}}\cdot\tilde{\boldsymbol{\nabla}}\tilde{\rho}|_{\tilde{R}} = 0 \,. \tag{18}$$

### B. Parameter estimates

Here we estimate parameter values from experimental data. The fixed parameters used in numerical simulations are presented in Table I.

- Membrane tension $\gamma_0 \sim 2-3$ $\mu$N/m [22], also used in Refs. [4, 23, 24] and others.
- Radius of contact zone $R \sim 5$ $\mu$m, similar to cell size.
- Equilibrium coverage - TCR: $c_R^0 \sim 200$ $\mu$m$^{-2}$, adhesion molecules (LFA): $c_A^0 \sim 2c_R^0 = 400$ $\mu$m$^{-2}$ [1].

- Protein receptor elastic stiffness (TCR-pMHC/BCR-antigen) $k_R \sim 24\ \mu$N/m and adhesion molecule stiffness (LFA1-ICAM1) $k_A \sim 164\ \mu$N/m, so $\kappa_0 = k_A c_A^0/(k_R c_R^0) \sim 13.7$ [3, 4].
- TCR-pMHC equilibrium length: $\ell_R \sim 15$ nm [1, 24].
- Glycoproteins/adhesion molecule length: $\ell_A \sim 40 - 45$ nm [1, 24].
- Average membrane separation $h_0 \sim (2\ell_1 + \ell_0)/3 \sim 35$ nm [1, 3, 24].
- Elastic strain and energy scales - for receptor: $\epsilon_0 = (h_0 - \ell_R)/h_0 \sim 0.5 - 0.6$ and $E_0 = k_R h_0^2/(2k_BT) \sim 3-4$, for adhesion molecule: $\epsilon_1 = (h_0 - \ell_A)/h_0 \sim -(0.1 - 0.3)$ and $E_1 = k_A h_0^2/(2k_BT) \sim 24 - 25$ ($k_BT = 4.1 \times 10^{-21}$ J at $T = 300$ K).
- Elasto-capillary length: $L_c \sim 0.1 - 0.3\ \mu$m, assuming $\rho_0 \sim 0.3 - 0.6$ similar to length scales obtained using bending rigidity [1].
- Receptor molecular diffusion $D_R \sim 0.5 - 1\ \mu\text{m}^2$/s [1, 3, 24].
- Hydrodynamic time scale $\tau_h \sim 2 \times 10^{-2} - 2$ s (using water viscosity $\eta = 10^{-3}$ Pa s and $L_c \sim 0.1 - 1\ \mu$m).
- Kinetic time $\tau_k \sim 10^{-5} - 10$ s (variable) [1, 3], so $\mathsf{Eh} \sim 10^{-3} - 10^5$.
- Binding affinity (variable depending on ligand): $K^A_{\rm eq} \sim 1 - 3$, $K^R_{\rm eq} \sim 0.1 - 3$ ($\rho_0 \sim 0.09 - 0.74$). [1, 3, 25].

| **Dimensionless parameter** | **Estimated value** |
|---|---|
| $D$ | 10 |
| $\mathsf{Eh}$ | 20 |
| $\epsilon_0$ | 0.6 |
| $\epsilon_1$ | $-0.3$ |
| $E_0$ | 3.6 |
| $E_1$ | 24.5 |
| $K^A_{\rm eq}$ | 1 |
| $\rho_0$ | 0.6 |
| $\kappa_0$ | 13.7 |
| $\theta$ | 4/3 |

TABLE I. List of fixed parameters used in numerical simulations. Exceptions: In Fig. 2E, we compare results obtained with $\mathsf{Eh} = 15, 20, 25, 30$. In Fig. 4, we study $\rho_0 \in [0.4, 0.7]$.

### C. Effective free energy and linear stability analysis

Here we analyze the nondimensional model (Eqs. 14-16) first by constructing an effective free energy like description in the $\mathsf{Pe} \ll 1$ limit and then performing a linear stability analysis of the homogeneous steady-state.

For weak contractility ($\mathsf{Pe} \ll 1$), there are no diffusive patterning instabilities in the receptor kinetics. We can then equilibrate $\tilde{\rho}$ to lowest order in gradients by setting $\tilde{\partial}_t \tilde{\rho} = 0$ and obtaining $\tilde{\rho}(\tilde{h}) \approx \tilde{\omega}_{\rm on}/[\rho_0(\tilde{\omega}_{\rm on} + \tilde{\omega}_{\rm off})] = 1/[\rho_0 + (1-\rho_0)e^{E_0(\tilde{h}-1)(\tilde{h}-1+2\epsilon_0)}]$. The slow dynamics of the height is then governed by an effective free energy $\mathcal{F} = \int {\rm d}\tilde{\mathbf{x}}\, [f(\tilde{h}) + |\tilde{\boldsymbol{\nabla}}\tilde{h}|^2/2]$ where the free energy density is given by

$$f(\tilde{h}) = \int_0^{\tilde{h}} {\rm d}h' \left[\rho(h')\left(h' - 1 + \epsilon_0 - \frac{A_\zeta}{[1 + \theta\tilde{\rho}(h')]}\right) + \frac{\kappa_0}{\rho_0}\frac{K^A_{\rm eq}(h' - 1 + \epsilon_1)}{[K^A_{\rm eq} + e^{E_1(h'-1+\epsilon_1)^2}]}\right] . \quad (19)$$

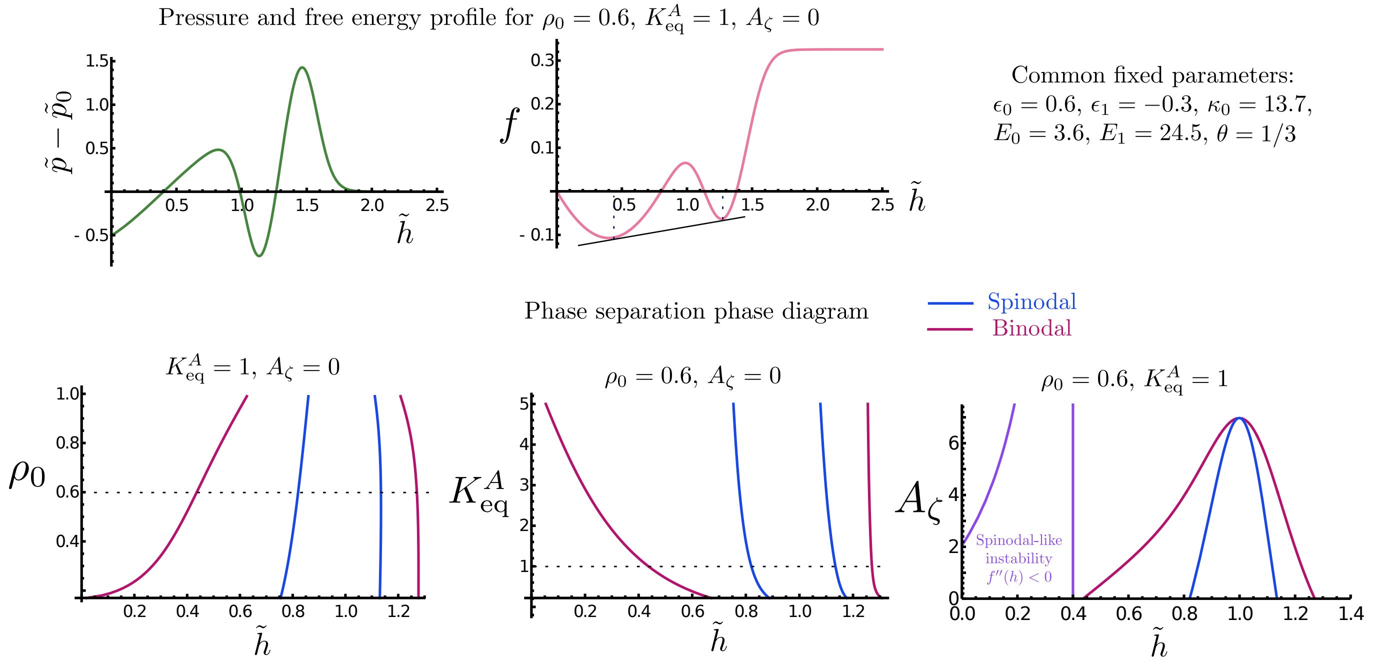


FIG. S1. Local pressure $\tilde{p}$ (no spatial gradients and $\tilde{p}_0$ is the $A_\zeta$ dependent constant offset) and free energy density $f$ shown as a function of $\tilde{h}$. Common tangent construction on $f(\tilde{h})$ determines the coexisting heights $\tilde{h}_{1,2}$ (binodal curve). Phase diagram with the binodal and spinodal curves shown for varying $\rho_0$, $K_{\rm eq}^A$ and $A_\zeta$. Increasing $\rho_0$ and $K_{\rm eq}^A$ affects the binodal curves more than the spinodal curves (larger change in the metastable region). Upon increasing $A_\zeta$ we eventually cross a critical point (akin to an upper consolute point) beyond which the system is stable to demixing at long-wavelengths. The $\tilde{h} = 1$ initial state is always in the spinodal regime, except for large $A_\zeta$. An additional spinodal-like unstable region ($f''(\tilde{h}) < 0$) is present at small $\tilde{h}$ when $A_\zeta > 0$. In the active case, other physically less-relevant instabilities are also present at larger heights ($\tilde{h} \gtrsim 1.5$, not shown).

Note constant shifts in the pressure (from $A_\zeta\langle m\rangle$) which lead to linear in $\tilde{h}$ terms in $f(\tilde{h})$ do not affect the coexistence conditions below. When $f(\tilde{h})$ in Eq. 19 has a double-well structure (plotted in Fig. S1), the proteins and membrane have a propensity to phase-segregate into domains. Following conventional phase-separation terminology, when $f''(\tilde{h}) < 0$, we have a spinodal instability, i.e., the system is diffusively unstable at long-wavelengths to spontaneous domain formation and coarsening (Fig. S1). In the case where $\int \mathrm{d}\tilde{\mathbf{x}}\ \tilde{h}$ is conserved, the coexisting densities/heights are given by the binodal curves. The binodals are computed through a standard common-tangent construction on $f(\tilde{h})$, i.e., the coexisting heights $\tilde{h}_{1,2}$ solve $f'(\tilde{h}_1) = f'(\tilde{h}_2)$ and $f(\tilde{h}_1) - f(\tilde{h}_2) = f'(\tilde{h}_1)(\tilde{h}_1 - \tilde{h}_2)$ (Fig. S1). Between the binodal and the spinodal curves the system is metastable and susceptible to finite amplitude perturbations (nucleation), see Fig. S1. In the current setting, due to fluid drainage through the boundary (so $\int \mathrm{d}\tilde{\mathbf{x}}\ \tilde{h}$ is not conserved), the final state is either a fully attached or fully detached state (and not a steady phase-separated state with partial attachment). Nonetheless, on a short time-scale, phase separation will drive transient pattern formation, with domains locally attaining the coexisting heights $\tilde{h}_{1,2}$. From Fig. S1, we clearly see that increasing $A_\zeta$ reduces the miscibility gap and raises the coexisting height (and associated receptor density) of the 'dilute phase' (lower binodal), consistent with our numerical simulation results.

While the free-energy provides a nonlinear characterization of the phase diagram, it only accounts for pulling active forces $A_\zeta$ and neglects $\mathsf{Pe}$ and the dynamics of $\tilde{\rho}$. To see when lateral activity ($\mathsf{Pe} > 0$) can drive instabilities, we disregard boundary conditions and linearize Eqs. 14-15 about the homogeneous steady-state $\tilde{h} = 1 + \delta h$, $\tilde{\rho} = 1 + \delta\rho$ (note this base state is a genuine steady-state of the equations in the bulk but it does not satisfy the boundary conditions as $\tilde{p} \neq 0$). This gives

$$\mathsf{Eh}\ \tilde{\partial}_t \delta h = (1+\kappa)\tilde{\nabla}^2\delta h - \tilde{\nabla}^4\delta h + \epsilon_0\tilde{\nabla}^2\delta\rho - \frac{A_\zeta}{(1+\theta)^2}\tilde{\nabla}^2\delta m\ , \tag{20}$$

$$\tilde{\partial}_t\delta\rho = -\delta\rho - 2(1-\rho_0)\epsilon_0 E_0\ \delta h + D\tilde{\nabla}^2\delta\rho - \frac{D\mathsf{Pe}}{(1+\theta)^2}\tilde{\nabla}^2\delta m + 2D\epsilon_0 E_0\tilde{\nabla}^2\delta h\ , \tag{21}$$

where $\kappa = (\kappa_0/\rho_0)K_{\rm eq}^A[K_{\rm eq}^A + \exp(E_1\epsilon_1^2)(1-2E_1\epsilon_1^2)]/[K_{\rm eq}^A + \exp(E_1\epsilon_1^2)]^2$ controls the elastic resistance to defor-

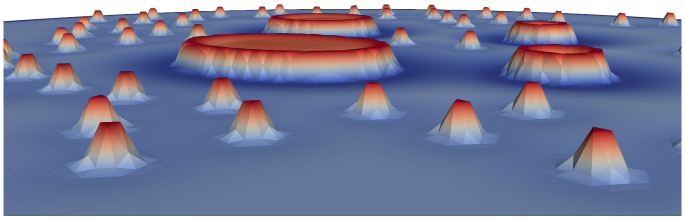

FIG. S2. Numerical resolution of the puncta in the finite-element solution of $\tilde{\rho}$ for the active case with $\mathsf{Pe} = 4.5$ and $A_\zeta = 0.25$.

mation due to the longer adhesion molecules. For the parameter values of interest (i.e., $h = 1$ lies in the spinodal region when passive), $1 + \kappa < 0$. Note that the linear stability equations would be unchanged upon including catch or slip bond behavior (Eqs. 11, 10). Keeping $k'_R/k_R \neq 1$, the steady-state still has $\rho = \rho_0 = K^R_{\rm eq}/[K^R_{\rm eq} + e^{E_0\epsilon_0^2}]$ independent of $k'_R$, and setting $\rho = \rho_0 + \delta\rho$ and $h = h_0 + \delta h$, the linearized kinetic rates give in Eq. 15, $\partial_t \delta\rho = -[\omega^R_{\rm on}(h_0) + \omega^R_{\rm off}(h_0)]\delta\rho + [(1-\rho_0)\partial_h\omega^R_{\rm on}(h_0) - \rho_0\partial_h\omega^R_{\rm off}(h_0)]\delta h + \mathcal{O}(\nabla^2)$. Noting $[\omega^R_{\rm on}(h_0) + \omega^R_{\rm off}(h_0)] = 1/\tau_k$, and $[\partial_h\omega^R_{\rm on}(h_0)/\omega^R_{\rm on}(h_0)] - [\partial_h\omega^R_{\rm off}(h_0)/\omega^R_{\rm off}(h_0)] = (k_R/k_BT)(\ell_R - h_0)$ is fully specified by detailed balance and is independent of $k'_R$, we have $\tau_k\partial_t\delta\rho = -\delta\rho - 2\rho_0(1-\rho_0)E_0\epsilon_0(\delta h/h_0) + \mathcal{O}(\nabla^2)$, confirming that catch/slip behavior leaves the linear analysis unchanged.

Substituting a Fourier spatial mode $(\delta h, \delta\rho) \sim e^{i\mathbf{q}\cdot\tilde{\mathbf{x}}}$ we convert the two coupled dynamical equations into a single second order equation in time for the height fluctuations that behaves like a linear damped harmonic oscillator, i.e.,

$$\delta\ddot{h} + \xi\delta\dot{h} + k\delta h = 0 \,, \tag{22}$$

$$\xi = \left[1 + q^2 D\left(1 - \frac{\mathsf{Pe}}{(1+\theta)^2}\right)\right] + \frac{q^2}{\mathsf{Eh}}(1 + \kappa + q^2) \,, \tag{23}$$

$$k = \frac{q^2}{\mathsf{Eh}}\left[(1+\kappa+q^2)\left(1 + q^2 D\left(1 - \frac{\mathsf{Pe}}{(1+\theta)^2}\right)\right) - 2\epsilon_0 E_0(1 - \rho_0 + Dq^2)\left(\epsilon_0 - \frac{A_\zeta}{(1+\theta)^2}\right)\right] \,, \tag{24}$$

where $q = |\mathbf{q}|$. Note, as $q \to \infty$, $\xi = q^4/\mathsf{Eh} + \mathcal{O}(q^2)$ and $k = (D/\mathsf{Eh})q^6[1 - \mathsf{Pe}/(1+\theta)^2] + \mathcal{O}(q^4)$. To ensure stability on short scales, we require $\xi, k > 0$ as $q \to \infty$, so $\mathsf{Pe} \leq \mathsf{Pe}_{\rm max} = (1+\theta)^2$. For our numerical simulation and state diagram (Fig. 2; main text), we are always below this threshold as $\mathsf{Pe}_{\rm max} = 5.44$ ($\theta = 4/3$), and our multifocal patterning instability occurs at a lower threshold at $\mathsf{Pe}_* \sim 4.25 < \mathsf{Pe}_{\rm max}$.

Plugging in the parameter values employed in the simulation (Table I), and considering $\delta h \sim e^{\sigma\tilde{t}}$ with growth rate $\sigma$, we find that there is always a positive growth rate corresponding to the diffusive height mode, so $\sigma = \sigma_2 q^2 - \sigma_4 q^4 + \mathcal{O}(q^6)$ with $\sigma_{2,4} > 0$. This yields a characteristic pattern wavelength at onset as in conventional spinodal instabilities with $q_* \sim \sqrt{\sigma_2/2\sigma_4}$ which only varies mildly as $q_* \sim 2 - 4$ when $\mathsf{Pe} \sim 0 - 5$ and $A_\zeta \sim 0 - 1$, and is already present even in the passive case ($\mathsf{Pe} = A_\zeta = 0$) So, we conclude that a linear analysis is insufficient to capture the observed transition from active coarsening to multifocal puncta.

## II. Numerical simulation methods

We fix the domain to be a circular disc $\Omega$ with radius $\tilde{R} = 50$. For the initial condition, we start with a random perturbation (of magnitude $\varepsilon$) around the homogeneous state $(\tilde{h}, \tilde{p}, \tilde{\rho}) = (1, 0, \rho_*)$ that satisfies the boundary conditions, so $\rho_* = (\kappa_0\epsilon_1/\epsilon_0\rho_0)(K^A_{\rm eq}/[K^A_{\rm eq} + e^{E_1\epsilon_1^2}])$, ensuring vanishing pressure. Note this initial state is *not* a steady-state of the model (as $\rho_* \neq 1$). Denoting $Z_1$ and $Z_2$ as two independent, uniformly distributed random variables in $[0, 1]$, we have as the initial condition,

$$\begin{aligned}\tilde{h}(\mathbf{x}, 0) &= 1 - \varepsilon Z_1 \,,\\ \tilde{p}(\mathbf{x}, 0) &= 0 \,,\\ \tilde{\rho}(\mathbf{x}, 0) &= \rho_* + \varepsilon Z_2 \,.\end{aligned}$$

Simulations are performed using the linear finite element method, implemented in FEniCSx (0.5.2) [26]. For time

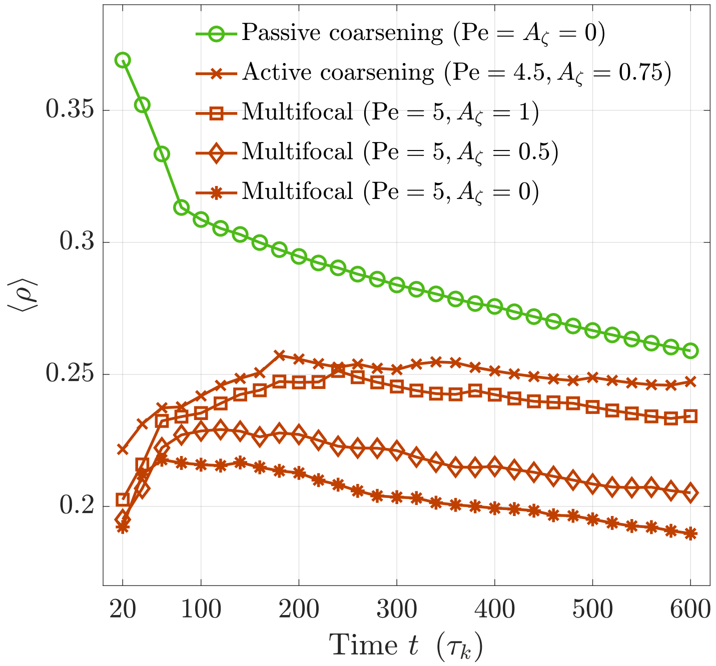


FIG. S3. Spatial average of the bound receptor fraction $\langle\rho\rangle$ as a function of time $t$ for the passive case and selected active scenarios. The corresponding curves for the cluster and background components are shown in Fig. 3 of the main text.

integration, we use the Backward Euler method with a fixed time step ranging from $\Delta t = 0.01$ to 0.1. We impose the constraint $0 \le \rho \le 1$ such that the bound receptor fraction is always positive and never exceeds one.

To accurately capture the formation and dynamics of localized structures, a sufficiently refined mesh is essential. We generate the meshes using the standard mesh generation package Gmsh [27]. The finest mesh consists of 57,337 nodes and 114,673 elements, with the longest edge of all triangles being 0.5430. With this level of numerical resolution, our solver is able to resolve the small puncta and track their motion. While we have checked that our solutions are qualitatively unchanged by varying mesh resolution, our current simulations are already computationally expensive. Each simulation takes 72–120 hours of wall-clock time, depending on the chosen time step. Further mesh refinement is computationally prohibitive.

## III. Post-processing

The post-processing tasks were performed in MATLAB [28]. In our simulations, an inhomogeneous pattern is first developed around $t = 20\tau_k$, when numerous well-separated domains emerge with values of $\rho$ significantly higher than those of the surrounding region. We identified these high-$\rho$ domains as receptor clusters and extracted them using the `contourf` function in MATLAB. Specifically, a cluster is identified as a region enclosed by a contour line at $\rho = 0.5/\rho_0$, and its size is measured as the area within this contour.

To analyze the overall dynamics of the synaptic pattern, we decompose the spatial average of the bound receptor fraction into two components, within clusters and in the background, respectively:

$$\langle\rho\rangle = \langle\rho\rangle_{\text{cluster}} + \langle\rho\rangle_{\text{background}}.$$

Here $\langle\rho\rangle_{\text{cluster}}$ denotes the spatial average of the $\rho$-field within all cluster regions, and $\langle\rho\rangle_{\text{background}}$ denotes the average outside the clusters. Hence, variations in $\langle\rho\rangle_{\text{cluster}}$ reflect changes in the clustered fraction of bound receptors, whereas variations in $\langle\rho\rangle_{\text{background}}$ capture changes in the background fraction.

To study the temporal dynamics of bound receptors, we fit quadratic curves to the simulated trajectories of $\langle\rho\rangle_{\text{cluster}}$ and $\langle\rho\rangle_{\text{background}}$ between $t = 20\tau_k$ and $t = 600\tau_k$. A comparison of these two components between passive and active cases is shown in main Fig. 6, while the time traces of the total bound fraction $\langle\rho\rangle$ are presented in Fig. S3.

To characterize the dependence of $\langle\rho\rangle_{\text{cluster}}$ and $\langle\rho\rangle$ on $K^R_{\text{eq}}$, we applied a quadratic fitting for passive and active cases, at $t = 100\tau_k$ and $t = 600\tau_k$, respectively. Simulation data were obtained at 10 equispaced values of $K^R_{\text{eq}}$ between

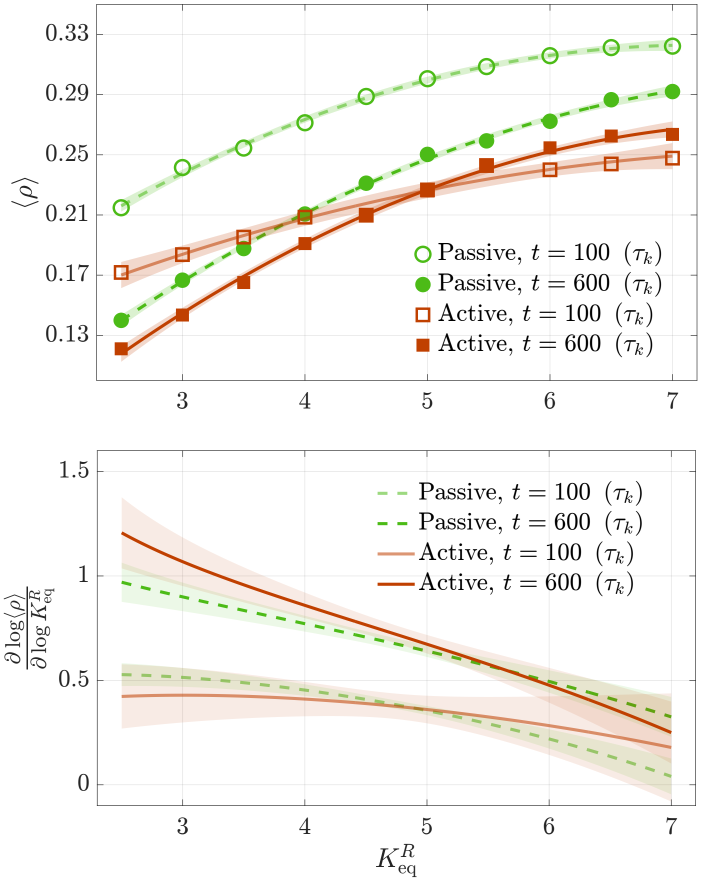


FIG. S4. Top: Spatial average of the bound receptor fraction $\langle\rho\rangle$ as a function of $K_{\rm eq}^R$. Lines are quadratic fit, with the shading indicating the 95% confidence interval. Bottom: Logarithmic sensitivity of $\langle\rho\rangle$ with respect to $K_{\rm eq}^R$, computed using Eq. (25). The corresponding plots for the cluster component are shown in Fig. 4 of the main text.

2.5 and 7. From the fitted quadratic curves, we computed the logarithmic sensitivity for $\langle\rho\rangle$

$$\frac{d\log\langle\rho\rangle}{d\log K_{\rm eq}^R} = \left[\frac{K_{\rm eq}^R}{\langle\rho\rangle}\right]\frac{d\langle\rho\rangle}{dK_{\rm eq}^R} \tag{25}$$

and analogously for $\langle\rho\rangle_{\rm cluster}$. The results for $\langle\rho\rangle_{\rm cluster}$ are shown in main Fig. 4, while the corresponding plots for $\langle\rho\rangle$ are presented in Fig. S4.

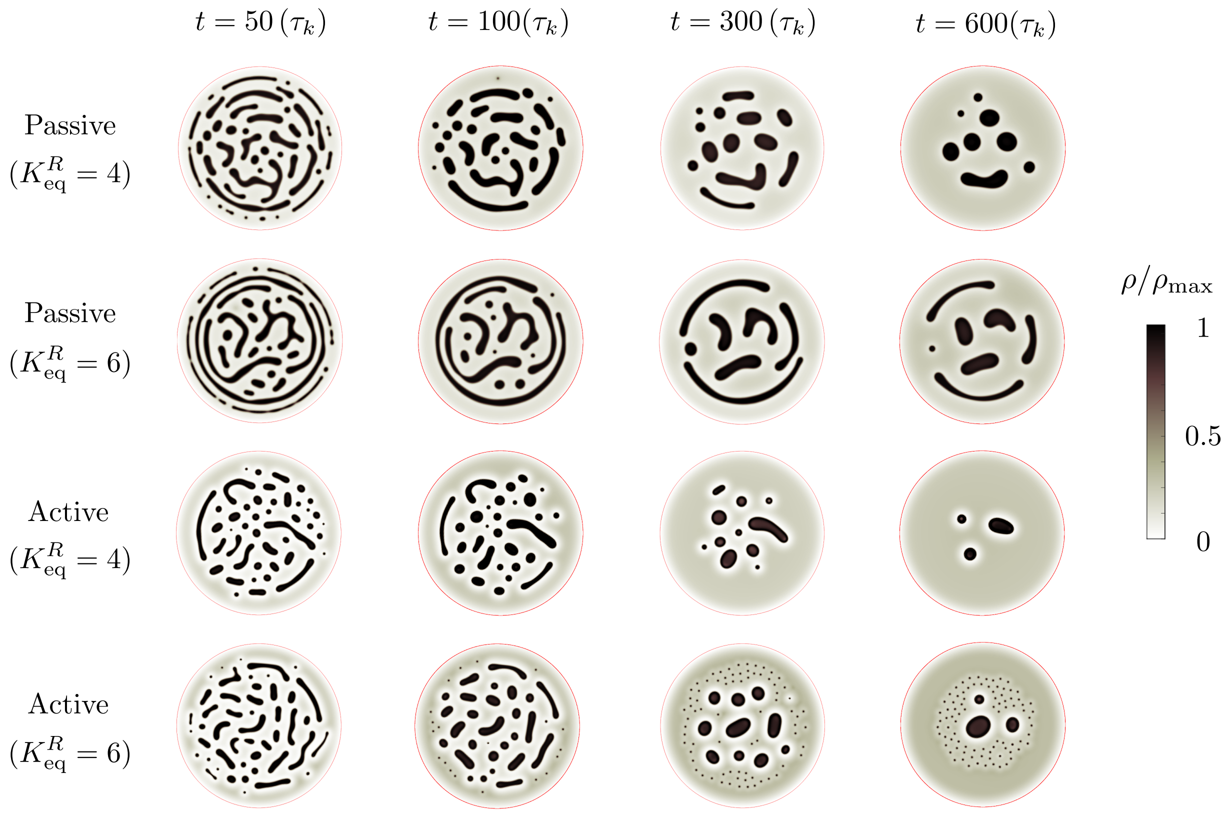


FIG. S5. Numerical solutions of the $\rho$ field in passive and active cases for $K^R_{\rm eq} = 4$ and $K^R_{\rm eq} = 6$ at the four labeled time points. Red circled patterns correspond to the two time points presented in Fig. 4 of the main text.

## IV. Supplementary Movies

**Movie 1.** Simulation video showing the time evolution of both the normalized membrane height ($\tilde{h} = h/h_0$) and the bound receptor fraction ($\tilde{\rho} = \rho/\rho_0$) in the passive case ($\mathsf{Pe} = A_\zeta = 0$) with $\mathsf{Eh} = 20$. The initial (random) density of bound receptors quickly coarsens: large domains grow, round up, and dissolve slowly into the background, while small clusters shrink and annihilate. Higher values of the membrane height ($\tilde{h} > 1$) reflect regions populated by an excess of longer adhesion molecules. The correspondence between low values of $\tilde{h}$ and high values of $\tilde{\rho}$ and vice versa reflects efficient segregation of short receptor-antigen complexes from long adhesion molecules.

**Movie 2.** Simulation video showing the time evolution of both the normalized membrane height ($\tilde{h} = h/h_0$) and the bound receptor fraction ($\tilde{\rho} = \rho/\rho_0$) in the active coarsening regime with $\mathsf{Pe} = 4.5$, $A_\zeta = 0.75$, and $\mathsf{Eh} = 20$. Under active forces, patterns coarsen faster than in the passive limit. While lateral contractility breaks down large domains, vertical pulling accelerates cluster dissolution and increases background receptor binding.

**Movie 3.** Simulation video showing the time evolution of both the normalized membrane height ($\tilde{h} = h/h_0$) and the bound receptor fraction ($\tilde{\rho} = \rho/\rho_0$) in the active multifocal clustering regime with $\mathsf{Pe} = 4.5$, $A_\zeta = 0.25$, and $\mathsf{Eh} = 20$. Here, strong contractility arrests coarsening and causes the larger clusters near the periphery to condense into localized puncta that remain stable instead of dissolving. Moreover, nascent puncta tend to emerge from the background near regions where cluster condensation occurs. Consequently, we observe long-lived multifocal localized patterns in the density field. Notably, these localized puncta do not significantly reduce the local membrane height; only larger clusters cause a considerable reduction in $\tilde{h}$.

[1] A. Carlson and L. Mahadevan, Elastohydrodynamics and kinetics of protein patterning in the immunological synapse, PLoS Computational Biology **11**, e1004481 (2015).

[2] A. Oron, S. H. Davis, and S. G. Bankoff, Long-scale evolution of thin liquid films, Review of Modern Physics **69**, 931 (1997).

[3] S. Qi, J. T. Groves, and A. K. Chakraborty, Synaptic pattern formation during cellular recognition, Proceedings of the National Academy of Sciences **98**, 6548 (2001).

[4] S. Raychaudhuri, A. K. Chakraborty, and M. Kardar, Effective membrane model of the immunological synapse, Physical Review Letters **91**, 208101 (2003).

[5] T. R. Powers, Dynamics of filaments and membranes in a viscous fluid, Reviews of Modern Physics **82**, 1607 (2010).

[6] J. Prost, F. Jülicher, and J.-F. Joanny, Active gel physics, Nature Physics **11**, 111 (2015).

[7] J.-F. Joanny and J. Prost, Active gels as a description of the actin-myosin cytoskeleton, HFSP Journal **3**, 94 (2009).

[8] G. Salbreux, G. Charras, and E. Paluch, Actin cortex mechanics and cellular morphogenesis, Trends in Cell Biology **22**, 536 (2012).

[9] A. G. Clark, K. Dierkes, and E. K. Paluch, Monitoring actin cortex thickness in live cells, Biophysical journal **105**, 570 (2013).

[10] A. Mogilner and A. Manhart, Intracellular fluid mechanics: Coupling cytoplasmic flow with active cytoskeletal gel, Annual Review of Fluid Mechanics **50**, 347 (2018).

[11] C. R. Nowosad, K. M. Spillane, and P. Tolar, Germinal center B cells recognize antigen through a specialized immune synapse architecture, Nature Immunology **17**, 870 (2016).

[12] S. R. De Groot and P. Mazur, *Non-equilibrium thermodynamics* (Courier Corporation, 2013).

[13] A. K. Chakraborty and A. Weiss, Insights into the initiation of tcr signaling, Nature Immunology **15**, 798 (2014).

[14] M. Dembo, D. Torney, K. Saxman, and D. Hammer, The reaction-limited kinetics of membrane-to-surface adhesion and detachment, Proceedings of the Royal Society of London. Series B. Biological Sciences **234**, 55 (1988).

[15] W. Chen, J. Lou, and C. Zhu, Forcing switch from short-to intermediate-and long-lived states of the $\alpha$a domain generates LFA-1/ICAM-1 catch bonds, Journal of Biological Chemistry **285**, 35967 (2010).

[16] W. Thomas, Catch bonds in adhesion, Annu. Rev. Biomed. Eng. **10**, 39 (2008).

[17] H.-K. Choi and C. Zhu, Catch bonds in immunology, Annual Review of Immunology **43** (2025).

[18] B. Liu, E. M. Kolawole, and B. D. Evavold, Mechanobiology of T cell activation: To catch a bond, Annual Review of Cell and Developmental Biology **37**, 65 (2021).

[19] A. Upadhyaya, Mechanosensing in the immune response, in *Seminars in cell & developmental biology*, Vol. 71 (Elsevier, 2017) pp. 137–145.

[20] P. Tolar, Cytoskeletal control of B cell responses to antigens, Nature Reviews Immunology **17**, 621 (2017).

[21] J. M. Brockman and K. Salaita, Mechanical proofreading: a general mechanism to enhance the fidelity of information transfer between cells, Frontiers in Physics **7**, 14 (2019).

[22] R. Simson, E. Wallraff, J. Faix, J. Niewöhner, G. Gerisch, and E. Sackmann, Membrane bending modulus and adhesion energy of wild-type and mutant cells of dictyostelium lacking talin or cortexillins, Biophysical Journal **74**, 514 (1998).

[23] M. Knežević, H. Jiang, and S. Wang, Active tuning of synaptic patterns enhances immune discrimination, Physical Review Letters **121**, 238101 (2018).

[24] T. R. Weikl and R. Lipowsky, Pattern formation during T-cell adhesion, Biophysical Journal **87**, 3665 (2004).

[25] Y. Tominaga, Y. Kita, A. Satoh, S. Asai, K. Kato, K. Ishikawa, T. Horiuchi, and T. Takashi, Affinity and kinetic analysis of the molecular interaction of ICAM-1 and leukocyte function-associated antigen-1, The Journal of Immunology **161**, 4016 (1998).

[26] I. A. Baratta, J. P. Dean, J. S. Dokken, M. Habera, J. S. Hale, C. N. Richardson, M. E. Rognes, M. W. Scroggs, N. Sime, and G. N. Wells, DOLFINx: the next generation FEniCS problem solving environment, preprint (2023).

[27] Geuzaine, Christophe and Remacle, Jean-Francois, Gmsh.

[28] T. M. Inc., Matlab version: 9.13.0 (r2022b) (2022).
